# Supplementary material for: Some comments on "On the generating function for intervals in Young's lattice" by Azam and Richmond
Source: arXiv:2401.04030 ancillary file (2025-02-05)
Supplement: Supplementary file 1 [file comment-azam-richmond.pdf]

# Some comments on “On the generating function for intervals in Young’s lattice” by Azam and Richmond

Jan Snellman

Azam and Richmond [1] obtained a recursion for the generating function of  $P_\lambda(y)$ , itself a generating function enumerating by length partitions in the lower ideal  $[0, \lambda]$  in the Young lattice. We show that this recursion can be extended to a multi-graded version. This is done by interpreting the original problem as enumerating plane partitions with two rows. We can then use the well-developed theory of lattice points in polyhedral cones to determine some properties of the generating function.

We also relate Azam and Richmond’s result to those obtained by Andrews and Paule in [2] using MacMahon’s  $\Omega$ -operator.

## 1 Introduction

In [1] Azam and Richmond considered the rank-generating function

$$P_\lambda(y) = \sum_{\mu \in [0, \lambda]} y^{|\mu|}$$

of the lower order ideal  $[0, \lambda]$  in the Young lattice. This is well-studied object, see [3], [4], and also [5].

The authors obtained a rational recursion for

$$Q_k(\mathbf{x}, y) = \sum_{\lambda \in \Lambda(k)} P_\lambda(y) \mathbf{x}^\lambda$$

where  $\Lambda(k)$  denotes the set of partitions with length  $k$ . They concluded that  $Q_k$  is a rational function, with denominator

$$D_k(x_1, \dots, x_k, y) = \prod_{m=1}^k \prod_{j=0}^m (1 - y^j \prod_{\ell=1}^m x_\ell).$$

These results were used to establish asymptotics for the average cardinality of lower order ideals  $[0, \lambda]$  of partitions  $\lambda$  of rank  $n$ .

In this note, we observe that

- replacing  $y^{|\mu|}$  with  $\mathbf{y}^\mu$ , thus using a multivariate  $P_\lambda(\mathbf{y})$ , and likewise for  $Q_k(\mathbf{x}, \mathbf{y})$ , allows us to rephrase the problem as counting plane partitions, or lattice points inside a polyhedral cone.
- This immediately shows that the generating function is rational, with the denominator given by the extremal rays of the cone.
- The rational recursion of [1] works for the multi-graded generating functions.
- Enumeration of plane partitions have been studied by many authors (see [6] and the references there); the methods of MacMahon [7]–[9], as expounded upon by Andrews and Paule [2], seems pertinent to the problem studied.

## 2 Multigradings, pairs of partitions, and plane partitions with two rows

### 2.1 The generating functions $Q_k$ and $\tilde{Q}_k$

Let us define

$$Q_k(\mathbf{x}, \mathbf{y}) = \sum_{\emptyset \leq \mu \leq \lambda \in \Lambda(k)} \mathbf{y}^\mu \mathbf{x}^\lambda.$$

Then specialising  $y_1 = y_2 = \dots = y_k = y$  we get back the previous  $Q_k(\mathbf{x}, y)$ .

Note that the multigraded version can be interpreted as the generating function of plane partitions with at most two rows, where the top row, representing  $\lambda$ , has  $\lambda_k > 0$ . Introducing

$$\tilde{Q}_k(\mathbf{x}, \mathbf{y}) = \sum_{\emptyset \leq \mu \leq \lambda \in \Lambda(\leq k)} \mathbf{y}^\mu \mathbf{x}^\lambda$$

where  $\Lambda(\leq k)$  denotes partitions with length at most  $k$ , we have that

$$\tilde{Q}_k = \sum_{j=0}^k Q_k$$

and that

$$Q_k = \tilde{Q}_k - \tilde{Q}_{k-1}.$$

**Example 1.** Let  $\lambda = (2, 1)$ . The lower order ideal  $[\emptyset, \lambda]$  contains

$$\emptyset, (1), (2), (1, 1), (2, 1)$$

and has multivariate generating function  $P_\lambda(\mathbf{y}) = 1 + y_1 + y_1^2 + y_1 y_2 + y_1^2 y_2$  which specialises to  $P_\lambda(y) = 1 + y + 2y^2 + y^3$ . The corresponding contribution to  $Q_k(\mathbf{x}, \mathbf{y})$ , for  $k \geq 2$ , is  $(1 + y_1 + y_1^2 + y_1 y_2 + y_1^2 y_2)x_1^2 x_2$ . These monomials can be regarded as plane partitions:

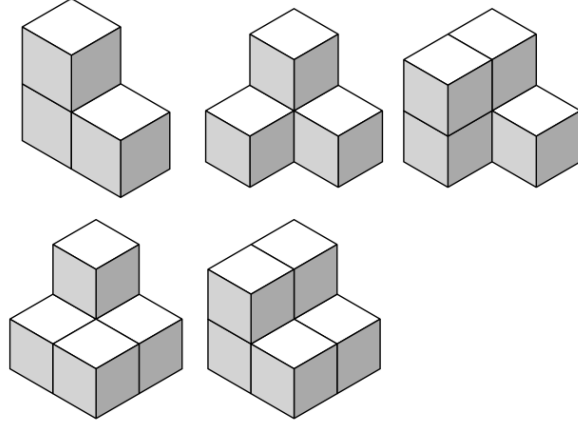

Figure 1: Plane partitions corresponding to monomials in generating function

## 2.2 Cones, hyperplanes, and polytopes

The generating function  $\tilde{Q}_k$  enumerates plane partitions contained in a 2-by- $k$  box. Explicitly, the inequalities that the integer vectors  $(\lambda, \mu) \in \mathbb{Z}^k \times \mathbb{Z}^k$  has to satisfy are as follows:

$$\lambda_i - \lambda_j \geq 0 \quad \forall i < j \quad (1)$$

$$\mu_i - \mu_j \geq 0 \quad \forall i < j \quad (2)$$

$$\lambda_i - \mu_i \geq 0 \quad \forall i \quad (3)$$

$$\lambda_i \geq 0 \quad \forall i \quad (4)$$

$$\mu_i \geq 0 \quad \forall i \quad (5)$$

We let  $C = C_k \subset \mathbb{R}^k \times \mathbb{R}^k$  denote the rational pointed polyhedral cone cut out in affine space by the above inequalities, and let  $A_k$  be its “integer transform”, that is to say, the affine monoid  $C_k \cap (\mathbb{Z}^k \times \mathbb{Z}^k)$ .

### 2.2.1 The case $k = 2$

For instance, when  $k = 2$ , the plane partitions in a  $2 \times 2$ -box are

$$\begin{pmatrix} \lambda_1 & \lambda_2 \\ \mu_1 & \mu_2 \end{pmatrix} \quad \lambda_1 \geq \lambda_2 \geq \mu_2 \geq 0, \lambda_1 \geq \mu_1 \geq \mu_2 \leq 0.$$

The corresponding integer transform is  $\tilde{Q}_2(x_1, x_2, y_1, y_2)$ ; to get the plane partitions enumerated by  $Q_2((x_1, x_2, y_1, y_2))$  we add the extra inequality  $\lambda_2 > 0$  (or  $\lambda_2 \geq 0$  if we prefer). The resulting polyhedron has  $C_2$  as its recession cone.

The cone  $C_2 \subset \mathbb{R}^2 \times \mathbb{R}^2$  has 5 extremal rays. We can calculate these using [10], [11].

Table 1: Generating rays of plane partitions inside a 2 by 2 box

|   |              |
|---|--------------|
| 0 | (1, 0, 0, 0) |
| 1 | (1, 0, 1, 0) |
| 2 | (1, 1, 0, 0) |
| 3 | (1, 1, 1, 0) |
| 4 | (1, 1, 1, 1) |

### 2.2.2 General $k$

For a general  $k$ , we note that all extremal rays of  $C = C_k$  intersect the affine hyperplane

$$H = \{(\lambda_1, \dots, \lambda_k, \mu_1, \dots, \mu_k) : \lambda_1 = 1\}$$

in lattice points. Call the set of these points  $S_k$ . Let  $P = P_k$  be the intersection  $C \cap H$ . Let  $T_k = P \cap (\mathbb{Z}^k \times \mathbb{Z}^k)$ . Recall that we introduced the affine monoid  $A = A_k = C_k \cap (\mathbb{Z}^k \times \mathbb{Z}^k)$  whose generating function is  $\tilde{Q}_k$ .

**Lemma 2.** *Let  $C_k, A_k, P_k, S_k, T_k$  be as above. Then*

1. *The cone  $C$  is the disjoint union*

$$C = \cup_{t \geq 0} tP$$

*of dilations of  $P$ .*

2.  $S_k = T_k$ .

3. *Denote the vector of length  $r$  consisting of all ones by  $\mathbf{1}^r$ , and the vector of length  $r$  consisting of all zeroes by  $\mathbf{0}^r$ . Put*

$$U_k = \{(\mathbf{1}^a, \mathbf{0}^b, \mathbf{1}^c, \mathbf{0}^d) : a + b = c + d = k, a \geq c, a \geq 1\}. \quad (6)$$

*Then  $S_k = T_k = U_k$ .*

4. The polytope  $P$  is the convex hull of  $S_k$ .
5.  $\tilde{Q}_k$  is the multigraded Ehrhart series of  $P$ .
6. Let  $D_k = \prod_{\mathbf{r} \in S_k} (1 - (\mathbf{x}\mathbf{y})^{\mathbf{r}})$ . Then  $\tilde{Q}_k \times D_k$  is a polynomial.
7.  $S_k$  form a Hilbert basis for the affine monoid  $A_k$ .

*Proof.* Let  $(\lambda, \mu)$  be a plane partition in  $A_k$ . If  $(\lambda, \mu)$  is nonzero, then  $\lambda_1 \geq 1$ . Let  $(s(\lambda), s(\mu))$  be the support of the pair; here  $s(\lambda)(i) = 1$  if  $\lambda_i > 0$ , and zero otherwise. Then it is easy to see that  $(s(\lambda), s(\mu)) \in U_k$ . Furthermore,

$$(\lambda, \mu) - (s(\lambda), s(\mu)) \in A_k.$$

Thus, every element in  $A_k$  is expressible as a sum of elements in  $U_k$ .

Elements in  $T_k$  are irreducible; if the partition  $(\mathbf{1}^a, \mathbf{0}^b)$  is to be written as a sum of elements in  $\mathbb{N}^k \times \mathbb{N}^k$ , one of the summands would have to start with a zero — but this is impossible.

By Gordan's lemma (see for instance [12]) we have that the Hilbert basis of  $A_k$  consists of the irreducible elements in the monoid. Any element in  $(\lambda, \mu) \in A_k$  with  $\lambda_1 > 1$  can be written as

$$(\lambda, \mu) = (s(\lambda), s(\mu)) + ((\lambda, \mu) - (s(\lambda), s(\mu)))$$

and is thus reducible. Hence, the Hilbert basis consists precisely of  $T_k$ , and this set is equal to  $U_k$  and  $S_k$ .  $\square$

For a simplicial rational cone, the generating function has numerator 1, and denominator given by the extremal rays. Our cone  $C$  is not simplicial, though; it has more generators than the embedding dimension  $2k$ . Thus the numerator is some multivariate polynomial. However, from general theory [12], [13], see also [14], [15] it follows that

**Corollary 3.** *The denominator of  $\tilde{Q}_k$ , and hence of  $Q_k$ , is precisely  $D_k$*

Specializing  $y_1 = \cdots = y_k = y$  we recover Proposition 15 of [1]. In the multigraded case there can be no cancellation between the numerator and the denominator of  $Q_k$ , so we can assert that this  $D_k$  is the denominator, not just divisible by the denominator.

## 2.3 Calculating $\tilde{Q}_k$ by triangulating $C_k$

### 2.3.1 $k = 2$

Let us consider  $C_2$  again. It lives in  $\mathbb{R}^2 \times \mathbb{R}^2$  but, as was shown in Table 1, it is spanned by 5 extremal rays, hence it is not simplicial. We can, however, triangulate it into a union of simplicial cones. Sagemath + Normaliz gives a triangulation:

$$(<0, 1, 2, 4>, <1, 2, 3, 4>)$$

So  $C = C_2 = K_1 \cup K_2$ , where  $K_1, K_2$  and  $K_3 = K_1 \cap K_2$  are rational simplicial cones.  $K_3$  is generated by the intersection of the generating rays of  $K_1$  and of  $K_2$ , that is to say, by  $r_1, r_1, r_4$ .

A rational polyhedral simplicial cone generated by the rays  $\mathbf{r}$  will have generating function

$$\frac{1}{\prod_{\mathbf{r}}(1 - (\mathbf{xy})^{\mathbf{r}})}.$$

Hence, by inclusion-exclusion,

$$\begin{aligned} & \frac{N}{(1 - (\mathbf{xy})^{r_0})(1 - (\mathbf{xy})^{r_1})(1 - (\mathbf{xy})^{r_2})(1 - (\mathbf{xy})^{r_3})(1 - (\mathbf{xy})^{r_4})} \\ &= \frac{1}{(1 - (\mathbf{xy})^{r_0})(1 - (\mathbf{xy})^{r_1})(1 - (\mathbf{xy})^{r_2})(1 - (\mathbf{xy})^{r_4})} \\ &+ \frac{1}{(1 - (\mathbf{xy})^{r_1})(1 - (\mathbf{xy})^{r_2})(1 - (\mathbf{xy})^{r_3})(1 - (\mathbf{xy})^{r_4})} \\ &- \frac{1}{(1 - (\mathbf{xy})^{r_1})(1 - (\mathbf{xy})^{r_2})(1 - (\mathbf{xy})^{r_4})} \end{aligned}$$

hence

$$N = (\mathbf{xy})^{r_3} + (\mathbf{xy})^{r_0} - (\mathbf{xy})^{r_0}(\mathbf{xy})^{r_3},$$

which evaluates to

$$(-x_0 y_0 x_1 + 1) + (-x_0 + 1) - (x_0^2 y_0 x_1 - x_0 y_0 x_1 - x_0 + 1) = -x_0^2 y_0 x_1 + 1$$

### 2.3.2 $k = 3$

**2.3.2.1 Plane partitions** For  $k = 3$  the plane partitions are

$$\begin{pmatrix} \lambda_1 & \lambda_2 & \lambda_3 \\ \mu_1 & \mu_2 & \mu_3 \end{pmatrix}$$

with inequalities ensuring that the entries are non-negative and non-increasing in rows and columns.

**2.3.2.2 Extremal rays** There are now 9 extremal rays, generating the cone  $C = C_3 \subset \mathbb{R}^3 \times \mathbb{R}^3$ .

**2.3.2.3 Triangulation** A (regular) triangulation is the following:

$$(<0, 1, 2, 4, 5, 8>, <0, 1, 4, 5, 7, 8>, <1, 2, 3, 4, 5, 8>, <1, 3, 4, 5, 6, 8>, <1, 4, 5, 6, 7, 8>)$$

Table 2: Extremal rays of plane partitions with 2 rows and 3 columns

|   |                    |
|---|--------------------|
| 0 | (1, 0, 0, 0, 0, 0) |
| 1 | (1, 0, 0, 1, 0, 0) |
| 2 | (1, 1, 0, 0, 0, 0) |
| 3 | (1, 1, 0, 1, 0, 0) |
| 4 | (1, 1, 0, 1, 1, 0) |
| 5 | (1, 1, 1, 0, 0, 0) |
| 6 | (1, 1, 1, 1, 0, 0) |
| 7 | (1, 1, 1, 1, 1, 0) |
| 8 | (1, 1, 1, 1, 1, 1) |

### 2.3.3 General $k$

It is feasible to use inclusion-exclusion to find  $\tilde{Q}_3$ , the generating function of the cone  $C_3$ . However, this is not an efficient way of calculating  $\tilde{Q}_k$  for general  $k$ . The number of extremal rays of  $C_k$  is, as we shown, equal to one less the number of plane partitions inside a  $2 \times k \times 1$  box. From [7], this number is  $\binom{2+k}{2} - 1$ . The number of simplicial subcones in the triangulation grows swiftly; it is equal to the Catalan number:

Table 3: nr of cones in triangulation of C

| k | dim(C) | number of rays | number of cones in triangulation |
|---|--------|----------------|----------------------------------|
| 2 | 4      | 5              | 2                                |
| 3 | 6      | 9              | 5                                |
| 4 | 8      | 14             | 14                               |
| 5 | 10     | 20             | 42                               |
| 6 | 12     | 27             | 132                              |
| 7 | 14     | 35             | 429                              |
| 8 | 16     | 44             | 1430                             |
| 9 | 18     | 54             | 4862                             |

## 3 The rational recursion of Azam and Richmond

### 3.1 Original version

We state the main result of [1]. Recall that their  $Q_k$  is multi-graded in  $\mathbf{x}$  but simply-graded in  $y$ , so depends on  $k + 1$  variables.

**Theorem 4** (Azam and Richmond Thm 1). *Let  $p_k = x_1 \cdots x_k$ , and for a sequence of parameters  $Z = (z_1, \dots, z_{k+1})$ , let*

$$Q_k(Z) = Q_k(z_1, \dots, z_k).$$

- *If  $Z = (x_1, \dots, x_k, y)$ , then denote  $Q_k = Q_k(Z)$ .*

- For  $0 < r \leq k$ , we put  $Z_r = (y^r p_{r+1}, x_{r+2}, x_{r+3}, \dots, x_k, y)$ .

Then  $Q_0 = 1$  and for  $k \geq 1$  we have

$$(1 - p_k)Q_k = x_k Q_{k-1} + \sum_{0 \leq i < r \leq k} \left( \frac{y^r p_k}{1 - y^r p_r} \right) Q_{k-r}(Z_r) \cdot Q_i \quad (7)$$

In particular,  $Q_k$  is a rational function in the variables  $x_1, \dots, x_k, y$ .

They go on to prove

**Proposition 5** (Azam and Richmond Proposition 15). *Let  $p_k = x_1 \cdots x_k$ , and  $D_k = D_k(x_1, \dots, x_k, y) = \prod_{m=1}^k \prod_{j=0}^m (1 - y^j p_m)$ . Then  $Q_k \cdot D_k$  is a polynomial.*

As we have seen, this latter result is a straight-forward consequence of classification of the generating rays of  $C_k$ .

### 3.1.1 Numerators $N_k(\mathbf{x}, y)$ of $Q_k(\mathbf{x}, y)$

We show the numerators  $N_k(\mathbf{x}, y) = D_k(\mathbf{x}, y)Q_k(\mathbf{x}, y)$ , as studied by Azam and Richmond, for  $k = 1, 2, 3$ . In the next section we will give multigraded versions. (For computer reasons we put  $y = y_0$ ).

$$N_1(x_1, y_0) = -y_0 x_1^2 + y_0 x_1 + x_1.$$

$$N_2(x_1, x_2, y_0) =$$

$$y_0^3 x_1^3 x_2^3 - y_0^3 x_1^2 x_2^2 - y_0^2 x_1^2 x_2^2 - y_0 x_1^2 x_2^2 + y_0^2 x_1 x_2 - y_0 x_1^2 x_2 + y_0 x_1 x_2 + x_1 x_2$$

$$N_3(x_1, x_2, x_3, y) =$$

$$\begin{aligned} & y_0^7 x_1^6 x_2^5 x_3^4 - y_0^7 x_1^5 x_2^4 x_3^3 - y_0^6 x_1^5 x_2^4 x_3^3 - y_0^6 x_1^4 x_2^4 x_3^4 \\ & - y_0^5 x_1^5 x_2^4 x_3^3 - y_0^4 x_1^5 x_2^4 x_3^3 + y_0^6 x_1^4 x_2^3 x_3^2 - y_0^4 x_1^5 x_2^4 x_3^2 \\ & + y_0^6 x_1^3 x_2^3 x_3^3 + y_0^5 x_1^4 x_2^3 x_3^2 + y_0^5 x_1^3 x_2^3 x_3^3 + 2y_0^4 x_1^4 x_2^3 x_3^2 \\ & + y_0^4 x_1^3 x_2^3 x_3^3 + y_0^3 x_1^4 x_2^3 x_3^2 + y_0^3 x_1^3 x_2^3 x_3^3 - y_0^5 x_1^2 x_2^2 x_3^2 \\ & + y_0^3 x_1^3 x_2^3 x_3^2 + y_0^2 x_1^4 x_2^3 x_3^2 - y_0^4 x_1^3 x_2^2 x_3 + y_0^3 x_1^3 x_2^3 x_3 \\ & - y_0^4 x_1^2 x_2^2 x_3^2 - 2y_0^3 x_1^2 x_2^2 x_3^2 - y_0^3 x_1^2 x_2^2 x_3 \\ & - y_0^2 x_1^2 x_2^2 x_3^2 - y_0^2 x_1^2 x_2^2 x_3 - y_0 x_1^2 x_2^2 x_3^2 + y_0^3 x_1 x_2 x_3 \\ & - y_0 x_1^2 x_2^2 x_3 + y_0^2 x_1 x_2 x_3 - y_0 x_1^2 x_2 x_3 + y_0 x_1 x_2 x_3 + x_1 x_2 x_3 \end{aligned}$$

## 3.2 Multigraded version

We come to the main purpose of this note: the rational recursion of  $Q_k$  works multigradedly!

**Corollary 6.** *For  $i, r, k \geq 0$ , define*

- $Q_k = Q_k(\mathbf{x}, \mathbf{y})$



- $p_r = x_1 \cdots x_r$
- $q_r = y_1 \cdots y_r$
- $\hat{Z}_{r,k} = (p_{r+1}q_r, x_{r+2}, \dots, x_k, y_{r+1}, \dots, y_k)$
- $R_{i,r,k} = \frac{p_k q_r}{(1-p_k)(1-p_r q_r)} Q_i Q_{k-r}(\hat{Z}_{r,k})$

Then  $Q_0 = 1$  and for  $k > 0$

$$Q_k = \frac{x_k Q_{k-1}}{1 - p_k} + \sum_{0 \leq i < r \leq k} R_{i,r,k} \quad (8)$$

*Proof (sketch).* The difference to the original theorem is that  $Q_k = Q_k(\mathbf{x}, \mathbf{y})$  is a function of  $2k$  variables whereas  $\mathbf{Q}_k(\mathbf{x}, y)$  is a function of  $k + 1$ . Furthermore, the substitution in  $Q_{k-r}$  is refined to

$$Q_{k-r}(x_1 \cdots x_{r+1} \cdot y_1 \cdots y_r, x_{r+2}, \dots, x_k, y_{r+1}, \dots, y_k)$$

rather than

$$Q_{k-r}(x_1 \cdots x_{r+1} \cdot y^r, x_{r+2}, \dots, x_k, y).$$

The various lemmas and propositions in Section 2 of [1] that prove the recursion are based on bijections, and can be modified so to work multigradedly. Specifically:

- Replace  $P_\lambda(y) = \sum_{\mu \in [\emptyset, \lambda]} y^{|\mu|}$  with  $P_\lambda(\mathbf{y}) = \sum_{\mu \in [\emptyset, \lambda]} \mathbf{y}^\mu$
- Replace  $P_{\mu, \lambda}(y) = \sum_{\nu \in [\mu, \lambda]} y^{|\nu|}$  with  $P_{\mu, \lambda}(\mathbf{y}) = \sum_{\nu \in [\mu, \lambda]} \mathbf{y}^\nu$
- Replace

$$Q_{k,m}(\mathbf{x}, y) = \sum_{\lambda \in \Lambda(k, m)} P_\lambda(y) \mathbf{x}^\lambda$$

with

$$Q_{k,m}(\mathbf{x}, \mathbf{y}) = \sum_{\lambda \in \Lambda(k, m)} P_\lambda(\mathbf{y}) \mathbf{x}^\lambda$$

- Proposition 12: Replace  $y^k$  with  $y_1 \cdots y_k$ .
- Proposition 14: Also replace

$$Q_{k-r, m-1}(y^r p_{r+1}, x_{r+2}, \dots, x_k, y) \text{ with } Q_{k-r, m-1}(q_r p_{r+1}, x_{r+2}, \dots, x_k, y_{r+1}, \dots, y_k)$$

- Lemma 13, Theorem 1: Do the above replacements.

□

### 3.2.1 Numerators $N_k(\mathbf{x}, \mathbf{y})$ for $k \leq 3$

The numerators  $N_k$  of  $Q_k = N_k/D_k$  are given below, for  $k = 1, 2, 3$ .

$$k = 1: -x_1^2 y_1 + x_1 y_1 + x_1.$$

$$k = 2: \begin{aligned} & x_1^3 y_1^2 x_2^3 y_2 - x_1^2 y_1^2 x_2^2 y_2 - x_1^2 y_1 x_2^2 y_2 - x_1^2 y_1 x_2^2 \\ & - x_1^2 y_1 x_2 + x_1 y_1 x_2 y_2 + x_1 y_1 x_2 + x_1 x_2 \end{aligned}$$

$$k = 3:$$

$$\begin{aligned} & x_1^6 y_1^4 x_2^5 y_2^2 x_3^4 y_3 - x_1^5 y_1^4 x_2^4 y_2^2 x_3^3 y_3 - x_1^5 y_1^3 x_2^4 y_2^2 x_3^3 y_3 \\ & - x_1^4 y_1^3 x_2^4 y_2^2 x_3^4 y_3 - x_1^5 y_1^3 x_2^4 y_2 x_3^3 y_3 - x_1^5 y_1^3 x_2^4 y_2 x_3^3 \\ & - x_1^5 y_1^3 x_2^4 y_2 x_3^2 + x_1^4 y_1^3 x_2^3 y_2^2 x_3^2 y_3 + x_1^3 y_1^3 x_2^3 y_2^2 x_3^3 y_3 \\ & + x_1^4 y_1^3 x_2^3 y_2 x_3^2 y_3 + x_1^3 y_1^2 x_2^3 y_2^2 x_3^3 y_3 + x_1^4 y_1^3 x_2^3 y_2 x_3^2 \\ & + x_1^4 y_1^2 x_2^3 y_2 x_3^2 y_3 + x_1^3 y_1^2 x_2^3 y_2 x_3^3 y_3 + x_1^4 y_1^2 x_2^3 y_2 x_3^2 \\ & + x_1^3 y_1^2 x_2^3 y_2 x_3^3 + x_1^4 y_1^2 x_2^3 x_3^2 + x_1^3 y_1^2 x_2^3 y_2 x_3^2 \\ & - x_1^2 y_1^2 x_2^2 y_2^2 x_3^2 y_3 + x_1^3 y_1^2 x_2^3 y_2 x_3 - x_1^3 y_1^2 x_2^2 y_2 x_3 y_3 \\ & - x_1^2 y_1^2 x_2^2 y_2 x_3^2 y_3 - x_1^2 y_1^2 x_2^2 y_2 x_3^2 - x_1^2 y_1 x_2^2 y_2 x_3^2 y_3 \\ & - x_1^2 y_1^2 x_2^2 y_2 x_3 - x_1^2 y_1 x_2^2 y_2 x_3^2 - x_1^2 y_1 x_2^2 y_2 x_3 \\ & - x_1^2 y_1 x_2^2 x_3^2 - x_1^2 y_1 x_2^2 x_3 + x_1 y_1 x_2 y_2 x_3 y_3 \\ & - x_1^2 y_1 x_2 x_3 + x_1 y_1 x_2 y_2 x_3 + x_1 y_1 x_2 x_3 + x_1 x_2 x_3 \end{aligned}$$

## 4 Relation to prior work by Andrews and Paule and MacMahon

### 4.1 Geometric interpretation of the rational recursion

The rational recursion above yields an efficient way of calculating  $Q_\ell$ , and hence  $\tilde{Q}_\ell$ . Explicitly,

$$\begin{aligned} \tilde{Q}_\ell &= \sum_{k=0}^{\ell} Q_k \\ &= \sum_{k=0}^{\ell} \left( \frac{x_k Q_{k-1}}{1 - p_k} + \sum_{0 \leq i < r \leq k} R_{i,r,k} \right) \\ &= \sum_{k=0}^{\ell} \left( \frac{x_k Q_{k-1}}{1 - p_k} + \sum_{0 \leq i < r \leq k} \frac{p_k q_r}{(1 - p_k)(1 - p_r q_r)} Q_i Q_{k-r}(\hat{Z}_{r,k}) \right) \end{aligned}$$

This is a description how to slice up the affine monoid  $A_\ell$  into disjoint pieces;  $Q_k$  enumerates lattice points in  $C \cap H^+$ ,  $C$  being the polyhedral cone, and  $H^+$  the open halfspace  $\lambda_k > 0$ . The term  $Q_{k-1} \frac{x_k}{1 - p_k}$  enumerates lattice points in the translation of the projection of  $C$  in a certain direction, et cetera. It is not a triangulation of  $C$  into

subcones, nor is it a “disjoint decomposition” as is computed by Normaliz; it is much more complicated.

## 4.2 Generating functions for plane partitions in a box using the $\Omega$ operator

In a series of papers, out of all which we will refer to [2], Andrews and Paule revisits MacMahon’s method of partition analysis. They define

$$p_{m,n}(X) = \sum_{a_{i,j} \in P_{m,n}} x_{1,1}^{a_{1,1}} \cdots x_{m,n}^{a_{m,n}}$$

where  $P_{m,n}$  consists of all  $m \times n$  matrices  $(a_{i,j})$  over non-negative integers  $a_{i,j}$  such that  $a_{i,j} \geq a_{i,j+1}$  and  $a_{i,j} \geq a_{i+1,j}$ . Putting  $m = 2$ , we get our objects of interest.

They then (pages 650-651) illustrate MacMahon’s method using his  $\Omega$  operator by calculating  $p_{2,2}(X)$ . This is of course the same as  $\tilde{Q}_2$ .

Their calculations start with introducing extraneous variables associated with the inequalities defining  $C_2$ :

$$\begin{aligned} p_{2,2}(X) &= \sum_{(a_{i,j}) \in P_{2,2}} x_{1,1}^{a_{1,1}} x_{1,2}^{a_{1,2}} x_{2,1}^{a_{2,1}} x_{2,2}^{a_{2,2}} \\ &= \Omega_{\geq} \sum_{a_{i,j} \geq 0} \lambda_{1,1}^{a_{1,1}-a_{1,2}} \lambda_{2,1}^{a_{2,1}-a_{2,2}} \mu_{1,1}^{a_{1,1}-a_{2,1}} \mu_{1,2}^{a_{1,2}-a_{2,2}} x_{1,1}^{a_{1,1}} x_{1,2}^{a_{1,2}} x_{2,1}^{a_{2,1}} x_{2,2}^{a_{2,2}} \\ &= \Omega_{\geq} \frac{1}{(1 - x_{1,1}\lambda_{1,1}\mu_{1,1})(1 - x_{2,1}\lambda_{2,1}/\mu_{1,1})(1 - x_{1,2}\mu_{1,2}/\lambda_{1,1})(1 - x_{2,2}/\lambda_{2,1}\mu_{1,2})} \end{aligned}$$

Then, the so-called “crude form” is transformed to the generating function.

We replicate their calculations using the Omega package (written by Daniel Krenn) in Sagemath. We could also have used the mathematica package [16] by Andrews et al, or the Maple package [17]. by Doron Zeilberger.

```
L.<mu11,mu12,l11,l21,x11,x12,x21,x22> = LaurentPolynomialRing(ZZ)
p22setup = [1-x11*l11*mu11,1-x21*l21/mu11,
            1-x12*mu12/l11,1-x22/(l21*mu12)]
p22=MacMahonOmega(l21,MacMahonOmega(
    l11,MacMahonOmega(mu12,MacMahonOmega(mu11,1,p22setup))))
[(_[0],_[1]) for _ in p22]

[(-x11^2*x12*x21 + 1, 1),
 (-x11 + 1, -1),
 (-x11*x12 + 1, -1),
 (-x11*x12*x21*x22 + 1, -1),
 (-x11*x21 + 1, -1),
 (-x11*x12*x21 + 1, -1)]
```

We recognize the numerator and denominator of  $\mathbf{Q}_2$ , with renamed variables.

The most interesting part, for us, in [2], is their Lemma 2.3, which provides a recursion for plane partitions in an  $m \times n$  box. Specialising to  $m = 2$  we get

**Corollary 7** (Andrews and Paule Lemma 2.3).

$$p_{2,n+1} \begin{pmatrix} x_{1,1} & \cdots & x_{1,n} & x_{1,n+1} \\ x_{2,1} & \cdots & x_{2,n} & x_{2,n+1} \end{pmatrix} = \left( 1 - x_{1,n+1}x_{2,n+1} \prod_{\substack{1 \leq i \leq 2 \\ 1 \leq j \leq n}} x_{i,j} \right)^{-1} \\ \times \Omega_{\geq} p_{2,n} \begin{pmatrix} x_{1,1} & \cdots & x_{1,n-1} & \lambda_0 x_{1,n} \\ x_{2,1} & \cdots & x_{2,n-1} & \lambda_1 x_{2,n} \end{pmatrix} \\ \times \frac{1}{\left(1 - \frac{x_{1,n+1}}{\lambda_0}\right) \left(1 - \frac{x_{1,n+1}x_{2,n+1}}{\lambda_0\lambda_1}\right)} \quad (9)$$

Without going into details regarding the  $\Omega$  operator, we will mention that it operates on formal Laurent polynomials and transforms the expression under its purvey so that the “spurious”  $\lambda$  variables (not related to partitions, we are using Andrews’ and Paule’s notations here) gets eliminated, and what is left is the desired generating function.

**Question 1.** *Is there a relation between the “rational recursion” (8) and Andrews’ and Paule’s recursion (9)?*

## 5 Affiliation

Jan Snellman  
Department of Mathematics  
Linköping University  
58183 Linköping, Sweden  
jan.snellman@liu.se

## 6 References

- [1] F. A. Azam and E. Richmond, “On the generating function for intervals in young’s lattice,” *The electronic journal of combinatorics*, pp. P2.16–P2.16, May 2023, doi: 10.37236/11407.
- [2] G. E. Andrews and P. Paule, “MacMahon’s partition analysis XII: Plane partitions,” *Journal of the london mathematical society*, vol. 76, no. 3, pp. 647–666, Dec. 2007, doi: 10.1112/jlms/jdm079.
- [3] D. Stanton, “Unimodality and young’s lattice,” *Journal of combinatorial theory, series a*, vol. 54, no. 1, pp. 41–53, May 1990, doi: 10.1016/0097-3165(90)90004-G.
- [4] Y. Ueno, “On the generating functions of the young lattice,” *Journal of algebra*, vol. 116, no. 2, pp. 261–270, Aug. 1988, doi: 10.1016/0021-8693(88)90217-7.

- [5] I. M. Gessel and N. Loehr, “Note on enumeration of partitions contained in a given shape,” *Linear algebra and its applications*, vol. 432, no. 2, pp. 583–585, Jan. 2010, doi: 10.1016/j.laa.2009.09.006.
- [6] C. Krattenthaler, “Plane partitions in the work of richard stanley and his school.” arXiv, May 15, 2015. doi: 10.48550/arXiv.1503.05934.
- [7] P. A. MacMahon, *Combinatory analysis*. Cambridge University Press, 1915.
- [8] P. A. MacMahon, “Memoir on the theory of the partitions of numbers. part II,” *Philosophical transactions of the royal society of london. series a, containing papers of a mathematical or physical character*, vol. 192, pp. 351–401, 1899, Accessed: Jan. 08, 2024. [Online]. Available: <https://www.jstor.org/stable/90784>
- [9] P. A. MacMahon, “Memoir on the theory of the partition of numbers. part i,” *Philosophical transactions of the royal society of london. series a, containing papers of a mathematical or physical character*, vol. 187, pp. 619–673, 1896, Accessed: Jan. 08, 2024. [Online]. Available: <https://www.jstor.org/stable/90716>
- [10] The Sage Developers, “SageMath, the sage mathematics software system (version 10.2),” manual, 2023.
- [11] W. Bruns, B. Ichim, C. Söger, and U. von der Ohe, “Normaliz. algorithms for rational cones and affine monoids,” manual, 2023.
- [12] W. Bruns and J. Gubeladze, “Affine monoids and their hilbert bases,” in *Polytopes, rings, and k-theory*, New York, NY: Springer New York, 2009, pp. 49–89. doi: 10.1007/b105283\_2.
- [13] A. Schrijver, *Theory of linear and integer programming*, Nachdr. in Wiley-interscience series in discrete mathematics and optimization. Chichester Weinheim: Wiley, 2011.
- [14] R. T. Firla and G. M. Ziegler, “Hilbert bases, unimodular triangulations, and binary covers of rational polyhedral cones,” *Discrete comput geom*, vol. 21, no. 2, pp. 205–216, Feb. 1999, doi: 10.1007/PL00009416.
- [15] J. A. De Loera, R. Hemmecke, and M. Köppe, *Algebraic and geometric ideas in the theory of discrete optimization*. Philadelphia, PA: Society for Industrial and Applied Mathematics, 2012. doi: 10.1137/1.9781611972443.
- [16] G. E. Andrews, P. Paule, and A. Riese, “MacMahon’s partition analysis: The omega package,” *European journal of combinatorics*, vol. 22, no. 7, pp. 887–904, Oct. 2001, doi: 10.1006/eujc.2001.0527.
- [17] D. Zeilberger, “LinDiophantus.txt: A maple package that finds generating functions representating solutions of systems of linear diophantine equations.” 2001. Accessed: Jan. 07, 2024. [Online]. Available: <https://sites.math.rutgers.edu/~zeilberg/tokhniot/LinDiophantus.txt>
